# Supplementary material for: Predicting Band Gaps with Hybrid Density Functionals
Source: arXiv:1608.04796 ancillary file (2016-10-06)
Supplement: Supplementary file 1 [file suppinfo.pdf]

# Supporting information for: “Predicting Band Gaps with Hybrid Density Functionals”

Alejandro J. Garza<sup>†,¶</sup> and Gustavo E. Scuseria<sup>\*,†,‡</sup>

*Department of Chemistry, Rice University, Houston, Texas 77251-1892, USA, and  
Department of Physics and Astronomy, Rice University, Houston, Texas 77251-1892, USA*

E-mail: guscus@rice.edu

We carried out band gap calculations for 41 semiconductors and insulators using the GAUSSIAN<sup>S1</sup> suite of programs. The set includes materials from the SC40 dataset,<sup>S2</sup> as well as transition metal oxides (FeO, CoO, NiO, MnO, and VO<sub>2</sub>) and large band gap salts (NaCl, LiCl, and LiF); the set is similar to that of Ref. S3 (some compounds have been excluded because spin-orbit effects are very large, and we have not used spin-orbit corrections in our calculations). As in that reference, we employed experimental geometries (references for the crystal structures may be found in the Supporting Information of Ref. S3). The basis sets used for SC40 compounds are the same as those of Ref. S2 (which are similar or identical to those in Ref. S3) and the basis sets of Ref. S3 are used for the rest of the compounds. However, while we had no problems to compute band gaps for all these compounds with HSE, some of the global hybrid calculations (particularly PBE0) were too expensive or too difficult

---

\*To whom correspondence should be addressed

<sup>†</sup>Department of Chemistry, Rice University, Houston, Texas 77251-1892, USA

<sup>‡</sup>Department of Physics and Astronomy, Rice University, Houston, Texas 77251-1892, USA

<sup>¶</sup>Present address: The Joint Center for Artificial Photosynthesis, Lawrence Berkeley National Laboratory, Berkeley, California 94720, USA

to converge. In cases when the calculation was too expensive with a global hybrid, we utilized the number of PBC matrices (the number of matrices used in the real-space representation of translational invariant one-body operators) from a converged HSE calculation as a starting point, then increased this number if problems arose in the diagonalization or to verify that it was large enough to adequately represent the band gap. Our results are summarized below.

| <b>Band Gaps</b> | <i>All values in eV. Omitted values represent convergence failure.</i> |            |               |              |             |  |
|------------------|------------------------------------------------------------------------|------------|---------------|--------------|-------------|--|
| <b>System</b>    | <b>Experiment</b>                                                      | <b>HSE</b> | <b>B3PW91</b> | <b>B3LYP</b> | <b>PBE0</b> |  |
| Ge               | 0.74                                                                   | 0.80       | 1.03          | 0.83         | 1.39        |  |
| Si               | 1.17                                                                   | 1.21       | 1.62          | 1.82         | 1.81        |  |
| $\beta$ -SiC     | 2.42                                                                   | 2.32       | 2.71          | 2.99         |             |  |
| BP               | 2.40                                                                   | 2.13       |               |              |             |  |
| AlP              | 2.50                                                                   | 2.42       | 2.85          | 3.06         | 3.07        |  |
| AlAs             | 2.23                                                                   | 2.13       | 2.56          | 2.75         | 2.77        |  |
| GaP              | 2.35                                                                   | 2.39       | 2.81          | 2.91         | 3.05        |  |
| GaAs             | 1.52                                                                   | 1.11       | 1.34          | 1.18         | 1.72        |  |
| GaSb             | 0.82                                                                   | 0.90       | 1.11          | 0.93         | 1.48        |  |
| InP              | 1.42                                                                   | 1.77       | 2.06          | 1.94         | 2.42        |  |
| InAs             | 0.42                                                                   | 0.57       | 0.76          | 0.61         | 1.12        |  |
| InSb             | 0.24                                                                   | 0.47       | 0.64          | 0.48         | 0.99        |  |
| ZnS              | 3.80                                                                   | 3.44       | 3.80          | 3.77         | 4.20        |  |
| ZnSe             | 2.82                                                                   | 2.38       | 2.70          | 2.64         | 3.09        |  |
| ZnTe             | 2.39                                                                   | 2.34       | 2.85          | 2.54         | 3.03        |  |
| CdSe             | 1.90                                                                   | 1.48       | 1.80          | 1.75         | 2.17        |  |
| CdTe             | 1.57                                                                   | 1.64       | 1.94          | 1.86         | 2.30        |  |
| $\beta$ -GaN     | 3.30                                                                   | 3.08       | 3.39          | 3.49         | 3.76        |  |
| $\alpha$ -GaN    | 3.50                                                                   | 3.48       | 3.80          | 3.89         | 4.17        |  |
| InN              | 0.72                                                                   | 0.72       | 0.98          |              |             |  |
| C                | 5.50                                                                   | 5.43       | 5.80          |              |             |  |
| AlSb             | 1.69                                                                   | 1.82       | 2.27          | 2.41         | 2.46        |  |
| BN               | 6.36                                                                   | 5.91       | 6.29          |              |             |  |
| CdS              | 2.55                                                                   | 2.21       |               |              | 2.95        |  |
| MgS              | 4.78                                                                   | 4.67       | 5.43          | 5.16         | 5.41        |  |
| MgTe             | 3.60                                                                   | 3.54       | 3.93          | 3.91         | 4.23        |  |
| AlN              | 6.19                                                                   | 5.74       |               |              |             |  |
| MgO              | 7.90                                                                   | 6.59       | 6.93          | 7.09         |             |  |
| BAAs             | 1.46                                                                   | 1.88       | 2.28          | 2.45         | 2.48        |  |
| MgSe             | 2.47                                                                   | 2.69       | 3.11          | 3.11         | 3.36        |  |
| BaS              | 3.88                                                                   | 3.19       | 3.65          | 3.69         | 3.95        |  |
| BaSe             | 3.58                                                                   | 2.74       | 3.20          | 3.25         | 3.47        |  |
| BaTe             | 3.08                                                                   | 2.21       | 2.68          | 2.75         | 2.92        |  |
| FeO              | 2.40                                                                   | 2.41       | 2.63          | 2.92         |             |  |
| CoO              | 2.50                                                                   | 2.82       | 3.06          | 3.14         |             |  |
| NiO              | 4.00                                                                   | 4.09       | 3.92          | 3.81         |             |  |
| MnO              | 4.00                                                                   | 4.77       | 4.79          | 4.56         |             |  |
| VO2              | 0.60                                                                   | 1.00       | 1.32          | 1.39         |             |  |
| NaCl             | 8.97                                                                   | 6.74       | 7.21          | 7.07         | 7.55        |  |
| LiCl             | 9.40                                                                   | 8.15       | 8.59          | 8.59         | 8.96        |  |
| LiF              | 14.20                                                                  | 13.28      |               |              |             |  |

## References

- (S1) Frisch, M. J.; Trucks, G. W.; Schlegel, H. B.; Scuseria, G. E.; Robb, M. A.; Cheeseman, J. R.; Scalmani, G.; Barone, V.; Mennucci, B.; Petersson, G. A. et al. *Gaussian 09*, Revision A.02; Gaussian Inc.: Wallingford, CT, 2009.
- (S2) Lucero, M. J.; Henderson, T. M.; Scuseria, G. E. Improved Semiconductor Lattice Parameters and Band Gaps from a Middle- Range Screened Hybrid Exchange functional. *J. Phys.: Condens. Matter* **2012**, *24*, 145504.
- (S3) Crowley, J. M.; Tahir-Kheli, J.; Goddard III, W. A. Resolution of the Band Gap Prediction Problem for Materials Design. *J. Chem. Phys. Lett.* **2016**, *7*, 1198–1203.
